# Supplementary material for: $U$-statistics on bipartite exchangeable networks
Source: arXiv:2103.12597 source file (2024-01-08)
Supplement: Supplementary file 3 [file appendix-mn.tex]

In this appendix, we provide the proofs for Proposition~\ref{prop:sequences} and further properties of the sequences $m_N$ and $n_N$ defined as $m_N = 2 + \lfloor c(N+1) \rfloor$ and $n_N = 2 + \lfloor (1-c)(N+1) \rfloor$ for all $N \geq 1$, where $c$ is an irrational number  (Definition \ref{def:mn}).

\begin{proof}[Proof of Proposition~\ref{prop:sequences}]
    The second result stems from the fact that 
    \begin{equation*}
        m_N + n_N = 4 + \lfloor c(N+1) \rfloor + \lfloor (1-c)(N+1) \rfloor = 4+\lfloor c(N+1) \rfloor + \lfloor -c(N+1) \rfloor + N+1
    \end{equation*}
    and $\lfloor c(N+1) \rfloor + \lfloor -c(N+1) \rfloor = -1$ because $c(N+1)$ is not an integer since $c$ is irrational. Then, the first result simply follows as
    \begin{equation*}
        \frac{m_N}{m_N + n_N} = \frac{\lfloor c(N+1) \rfloor + 2}{N + 4} \underset{N}{\sim} \frac{c(N+1) + 2}{N + 4} \underset{N}{\sim} \frac{cN}{N},
    \end{equation*}
    where $\underset{N}{\sim}$ denotes the asymptotic equivalence when $N$ grows to infinity, i.e. $a_N \underset{N}{\sim} b_N$ if and only if $a_N / b_N \underset{N \rightarrow \infty}{\longrightarrow} 1$.
\end{proof}

\begin{proof}[Proof of Corollary~\ref{cor:partition}]
    As $m_N$ and $n_N$ are non decreasing, the corollary is a direct consequence of $m_N + n_N = 4 + N$, because then $m_{N+1} + n_{N+1} = 4 + N + 1 = m_N + n_N + 1$.
\end{proof}

\begin{definition}
    We define $\mathcal{B}_c$ and $\mathcal{B}_{1-c}$ two complementary subsets of $\mathbb{N}^*$ as
    \begin{equation*}
        \mathcal{B}_c = \left\{ N \in \mathbb{N}^* : m_N = m_{N-1} + 1 \right\} \text{~and~~} \mathcal{B}_{1-c} = \left\{ N \in \mathbb{N}^* : n_N = n_{N-1} + 1 \right\}.
    \end{equation*}
    \label{def:partition_sets}
\end{definition}

\begin{proposition}
    Set $\kappa_c(m) := \big\lfloor \frac{m-2}{c} \big\rfloor$ and $\kappa_{1-c}(n) := \big\lfloor \frac{n-2}{1-c} \big\rfloor$. If $N \in \mathcal{B}_c$, then $N = \kappa_c(m_N)$. Similarly, if $N \in \mathcal{B}_{1-c}$, then $N = \kappa_{1-c}(n_N)$.
    \label{prop:form_k_m}
\end{proposition}

\begin{proof}
  Remember that $c$ is an irrational number, so if $N \in \mathcal{B}_c$, then
  \begin{equation*}
        cN + 2 < \lfloor cN \rfloor + 3 = m_{N-1} + 1 = m_N = \lfloor c(N+1) \rfloor + 2 < c(N+1) + 2,
    \end{equation*}
    which means that $\frac{m_N-2}{c} -1 < N < \frac{m_N-2}{c}$, thus $N = \big\lfloor \frac{m_N-2}{c} \big\rfloor$.
\end{proof}
